# Supplementary material for: Apparent remote synchronization of amplitudes: a demodulation and interference effect
Source: arXiv:1802.09380 source file (2018-06-23)
Supplement: Supplementary file 1 [file supplementary.pdf]

## SUPPLEMENTARY RESULTS

## I. TRANSITIONS AND EFFECT OF PARAMETRIC MISMATCHES

As reported in Ref. 15, the gains $G_6$ and $G_\mathrm{i}$ respectively control the internal loop gain and coupling strength of each oscillator with the preceding one on the ring, and act as the main control parameters, whereas the integration constant $K_1$ acts an additional control parameter. As a function of these control parameter settings, three dynamical regimes featuring different frequency spectra are observed in this system: quasiperiodicity, "fully-developed" chaos and a form of "weaker" chaos. These were characterized, respectively, by a comb-like spectrum of delta functions, a broadband spectrum without distinct peaks, and an intermediate spectrum with narrow peaks, broader than delta functions but well-separated. Remote synchronization was observed only for the third case, which is close to quasiperiodicity and wherein chaoticy was manifest in the form of relatively constrained amplitude fluctuations. Since in Ref. 15 route-to-chaos analysis was not performed and the largest Lyapunov's exponent was not calculated, there remains the question whether the system is truly chaotic in such state, or the corresponding broad peaks more trivially reflect the parametric mismatches.

To address this issue, simulations were performed for a ring of $n = 32$ nodes, sweeping the control parameters $G_6$, $G_\mathrm{i}$ and $K_1$ and generating bifurcation diagrams from the local maxima. As in Ref. 15, for observing remote synchronization in the simulations we set $G_6 = 0.188$ and $G_\mathrm{i} = -1.14$, and separately swept $G_6 \in [0.16, 0.25]$ (Fig. S1a), $-G_\mathrm{i} \in [0.9, 1.5]$ (Fig. S1b) and $K_1 \in [0.077, 0.143]$ $\mu\mathrm{s}^{-1}$ (Fig. S1c). As a function of all three control parameters, period doubling and subsequent transition to chaos were clearly observed, followed by a sudden change in the size of the chaotic attractor, also known as an interior crisis[55]. The corresponding largest Lyapunov exponent $\lambda_\mathrm{max}$ was estimated using Kantz's method ($\Delta t = 1\mu s$, 250,000 pts.)[59]. Prior to the crisis, i.e. for the regime associated with remote synchronization ($G_6 = 0.188$, $G_\mathrm{i} = -1.14$), we measured $\lambda_\mathrm{max} = 0.0032 \pm 0.0004$. After the crisis, i.e. for the regime yielding the broadband frequency spectrum ($G_6 = 0.196$, $G_\mathrm{i} = -1.365$), we measured $\lambda_\mathrm{max} = 0.0045 \pm 0.0008$.

These results confirm that when remote synchronization is observed in this system the underlying dynamics are indeed chaotic, however there remains the question of what influence the presence of parametric mismatches has on the emergence of this state. To address this issue, additional simulations were performed sweeping $\xi \in [10^{-18}, 10^{0}]$ (Fig. S1d). We observed that for $\xi \in [10^{-17}, 10^{-3}]$, remote synchronization reliably emerges with negligible dependence on $\xi$. Contrariwise, for $\xi \leq 10^{-18}$ and $\xi \geq 10^{-2}$ two qualitatively different states are observed, respectively characterized by global synchronization and by partial synchronization without remoteness (i.e. monotonic synchronization decay with distance). Except for the auxiliary system in Section V, identical initial conditions $v_1 = 1$ V, $v_2 = v_3 = v_4 = v_5 = v_6 = 0$ were always used; these settings are not critical, and heterogeneities in the initial conditions have an effect akin to that of parametric mismatches (data not shown). These results indicate that, even though the state of remote synchronization has a large basin of attraction, three states actually coexist[56]. Parametric mismatches are therefore necessary to provide some level of repulsion allowing activity to become differentiated across nodes. However, when they are too large they overwhelm the non-linear mechanism of energy exchange between frequency bands underlying the effect (see Section VII), and simpler synchronization phenomena prevail. It is noted that the tolerances estimated for the physical system, i.e. $\xi = 0.005$, are close to the upper bound for which remote synchronization emerges. More generally, remote synchronization requires parameter settings sustaining the interference effect reported in Section VII, whereas global synchronization and partial synchronization without remoteness arise over extended regions. Sharp transitions between the three states can be observed particularly as a function of gains $G_2$ and $G_3$ (data not shown).

## II. REVISED GRANGER CAUSALITY ANALYSIS

As discussed in Sections VI and VII, in the simplified chain model synchronization dips at a certain distance from a starting node due to destructive interference between the lower sideband (low frequency activity preexisting in the input signal) and the demodulated baseband (generated locally). This superposition almost completely cancels out the amplitude fluctuations (envelope) for which remote synchronization is observed in this system.

Importantly, in the full ring each node acts not only as a relay but also as an "active" generator of an own signal, therefore such effect is found in a "staggered" arrangement, wherein each node simultaneously processes the signals from multiple previous nodes located at different distances. This turns the synchronization dip and subsequent recovery observed for the chain model (Fig. 7a) into the diagonal pattern visible to the correlation, mutual information and linear causality analyses (Fig. 2c and Fig. 3a,b).

Having previously established that the lower sideband and the baseband are spectrally coincident, extracting the former via low-pass filtering should reveal correlation and causality patterns reflecting the results originally obtained for amplitude fluctuations, determined using Hilbert's transform as detailed in Subsection II. This hypothesis is founded on the notion that the two spectrally overlapped signals are the primary components in the interaction between nodes.

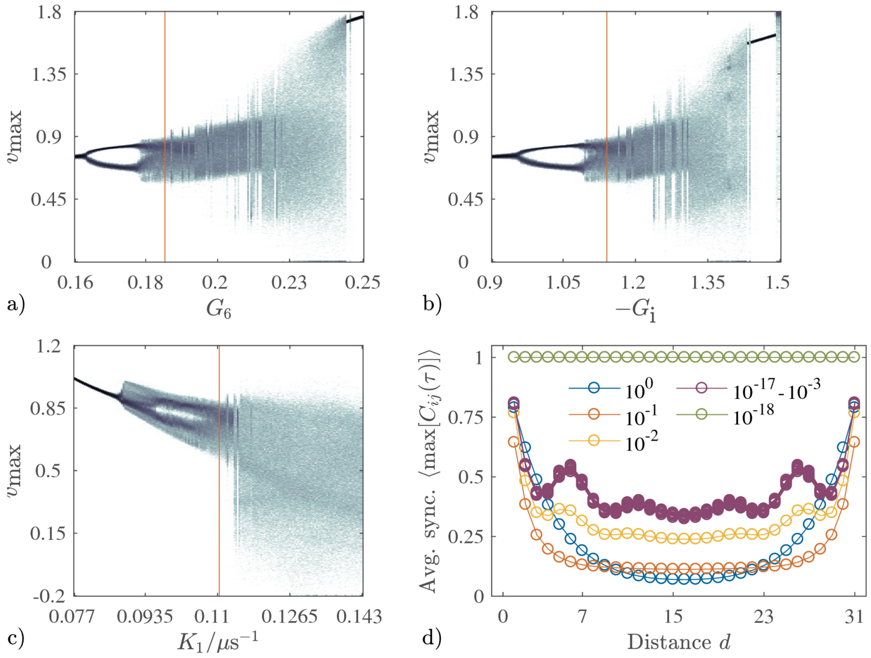


FIG. S1. Control parameter sweep and mismatch level simulations. a), b) and c) Bifurcation diagrams showing the local maxima distribution as a function of the control parameters $G_6$, $G_{\mathrm{i}}$ and $K_1$, revealing transition to chaos and subsequent crisis. Red bars denote parameter settings chosen for observing remote synchronization, logarithmic gray-scale. d) Average amplitude synchronization as a function of distance along the ring, delineating the basin of attraction of the remotely-synchronized state (purple plot, peak at $d = 6$) as a function of the parameter mismatch level $\xi$. See Supplementary Section I for detailed description.

To verify this hypothesis, the signals from the initial experiments were processed through a low-pass FIR filter having $f_{\mathrm{pass}} = 2.0$ kHz and $f_{\mathrm{stop}} = 2.5$ kHz, passband ripple 0.1 dB, stopband attenuation 40 dB (Fig. S2a). In order not to confound causality in these analyses, zero-phase digital filtering was performed (leading to squared transfer function and doubled filter order). While filtering to isolate causal influences within specific frequency bands can be problematic[57,58] and is theoretically unnecessary[57], for the present purpose it was deemed appropriate since there was a strong prior to confirm the previous analysis and need to prevent the much stronger carrier frequency from overwhelming the low-frequency dynamics. For consistency, the same settings as in Section III were kept, namely $\tau = 0.18$ ms, $p = 16$, $\delta = 1/f_{\mathrm{s}} = 0.01$ ms and $d \in [0, 2]$ ms. As expected, applying the Granger linear model in Eq. (9) to the resulting signal yielded a causality pattern closely resembling the one previously obtained for the envelope signal (Fig. S2b).

As described in Subsection VII B, in the simplified chain model, at the point of synchronization dip, the "hidden" synchronization information could be recovered by applying a peaking filter to emphasize the higher sideband and carrier with respect to the lower sideband, and then extracting the envelope. This is because, as also confirmed by simulations on the insertion of filters in the chain, at that point the synchronization information is conveyed predominantly through the higher sideband, since the lower sideband is almost completely nulled. It should therefore be possible to apply a similar approach to "plug" the diagonal line of desynchronization observed in the full ring.

For this purpose, the initial experimental signals were filtered using a second-order peaking filter having manually chosen $f_0 = 3.65$ kHz and $Q = 3$ (Fig. S2a), and the envelope of this signal was considered. In the resulting causality pattern, remoteness was considerably less evident and the information transfer more closely followed a monotonic decay (Fig. S2c).

Even though destructive interference primarily affected the lower sideband so that more predictive information was conveyed by the higher sideband, due to the nonlinearity there is a mutual interdependence between the two, which in the full ring is further complicated by the "active" role of each node. It is therefore reasonable to speculate that the lower sideband signals may contain predictive information not present in the higher sideband signals, or even that synergistic interaction between the lower sideband and the envelope of the higher sideband may take place, giving rise to predictive information that is available only taking both regressors together. Exploring this possibility, a final analysis was conducted simultaneously including into the regressors the activity of both sidebands. The resulting causality matrix revealed markedly stronger information transfer, without any residual aspect of remoteness (Fig. S2d).

Taken together, these findings demonstrate that a linear causality model is capable of resolving the underlying information transfer, insofar as the activity of both sidebands is represented in a manner appropriate for the system, in this case through filtering and demodulating the higher sideband. This is the relationship which could be approximated by the quadratic Granger model and agnostically captured by the model-free transfer entropy analysis reported in Section III.

[55]C. Grebogi, E. Ott and J. A. Yorke, *Crises, sudden changes in chaotic attractors, and transient chaos*, Physica D. **7** (1983) (1),

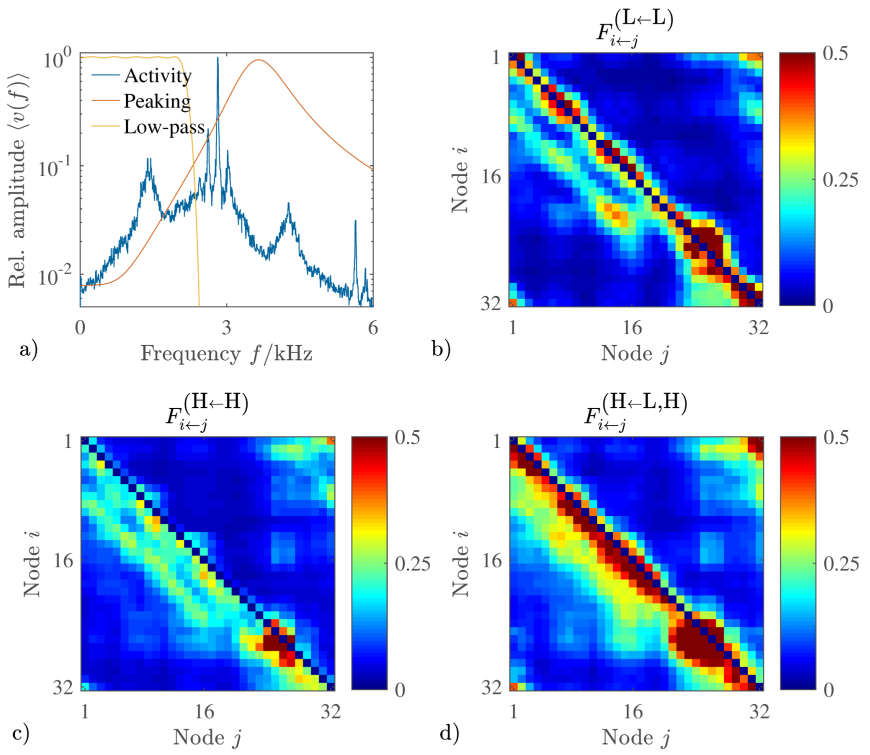


FIG. S2. Granger causality analyses for the lower sideband (L) and baseband demodulated from the filtered higher sideband (H). a) Average frequency spectrum of the experimentally-measured signals (normalized to unit maximum), and amplitude responses of the chosen low-pass and peaking filters. b) Granger causality for the lower sideband (L). c) Granger causality for the demodulated baseband, i.e. envelope of the higher sideband extracted via the peaking filter (H). d) Granger causality according to a model merging the predictors (L,H) considered in b) and c). See Supplementary Section II for detailed description.


pp. 181 – 200

[56] P. J. Menck, J. Heitzig, N. Marwan and J. Kurths, *How basin stability complements the linear-stability paradigm*, Nat. Phys. **9** (2013), pp. 89 – 92

[57] L. Barnett and A. Seth, *Behaviour of Granger causality under filtering: Theoretical invariance and practical application*, J. Neurosci. Methods **201** (2011) (2), pp. 404–419

[58] E. Florin, J. Gross, J. Pfeifer, G. R. Fink and L. Timmermann, *The effect of filtering on Granger causality based multivariate causality measures*, NeuroImage **50** (2010) (2), pp. 577 – 588

[59] H. Kantz, *A robust method to estimate the maximal Lyapunov exponent of a time series*, Phys. Lett. **185** (1994) (1), pp. 77 – 87
